# Supplementary material for: Intrinsic mechanism for anisotropic magnetoresistance and experimental confirmation in Co$_x$Fe$_{1-x}$ single-crystal films
Source: arXiv:2008.00872 source file (2020-08-03)
Supplement: Supplementary file 1 [file CoFe_AMR_Supplemental_rev3.pdf]

**Supplemental Materials for**

# Intrinsic mechanism for anisotropic magnetoresistance and experimental confirmation in $Co_xFe_{1-x}$ single-crystal films

F. L. Zeng, Z. Y. Ren, Y. Li, J. Y. Zeng, M. W. Jia, J. Miao, A. Hoffmann, W. Zhang, Y. Z. Wu and Z. Yuan

## I. First-principles transport calculations

Based on density functional theory, the electronic structure was self-consistently calculated for a slab of $Co_xFe_{1-x}$ alloy sandwiched by two semi-infinite Fe leads using a surface Green's function method implemented with tight-binding linear muffin-tin orbitals [S1]. To model the substitutional alloy, the charge densities and potentials inside the Fe and Co atomic spheres were obtained using the coherent potential approximation. In the transport calculation, the resulting atomic sphere potentials were then assigned randomly to sites in the 4x4 lateral supercells subject to maintenance of the appropriate concentration of the alloy and spin-orbit coupling is included in the Hamiltonian. Periodic boundary condition was applied in the lateral directions. The exchange potentials were rotated in spin space according to the required magnetization orientation. Then we determine all the incoming, $\boldsymbol{I}$ ($\boldsymbol{I'}$), and outgoing, $\boldsymbol{O}$ ($\boldsymbol{O'}$), propagating Bloch states in the left (right) lead, which were written in the vector form with the size equal to the number of states. All these states are connected by the scattering matrix $\boldsymbol{S}$, which is made up of reflection $\boldsymbol{r}$ ($\boldsymbol{r'}$) and transmission $\boldsymbol{t}$ ($\boldsymbol{t'}$) matrices, i.e.

$$\begin{pmatrix}\boldsymbol{O}\\ \boldsymbol{O}'\end{pmatrix} = \begin{pmatrix}\boldsymbol{r} & \boldsymbol{t}'\\ \boldsymbol{t} & \boldsymbol{r}'\end{pmatrix}\begin{pmatrix}\boldsymbol{I}\\ \boldsymbol{I}'\end{pmatrix} = \boldsymbol{S}\begin{pmatrix}\boldsymbol{I}\\ \boldsymbol{I}'\end{pmatrix}.$$

The scattering matrix was determined using the "wave-function matching" technique and evaluated at the Fermi level [S2]. Within the Landauer-Büttiker scattering formalism, the conductance $G$ (or resistance $R$) of the system was obtained via

$$R = G^{-1} = \left[\frac{e^2}{h}\mathrm{Tr}\left(\boldsymbol{t}\boldsymbol{t}^{\dagger}\right)\right]^{-1}.$$

For disordered alloys, a number of random configurations were computed until the average value and the variance converged with respect to the number of configurations. Then, by varying the length of the substitutional $Co_xFe_{1-x}$ alloy, we were able to extract the corresponding resistivity. Our Landauer-Büttiker formalism is found to be equivalent to the Kubo theory [S3]. Such equivalence has been explicitly demonstrated by the consistency of both bulk resistivity and Gilbert

damping calculated using the Kubo-based methods [S4, S5] and the Landauer-Büttiker formalism [S2, S6].

## II. Correlation between AMR and crossing bands

In the main text, we associated the anisotropic magnetoresistance (AMR) with the variations of band crossing/anticrossing depending on the magnetization direction. Here we take pure Fe as an example to explicitly illustrate the direct relationship between AMR and band structure.

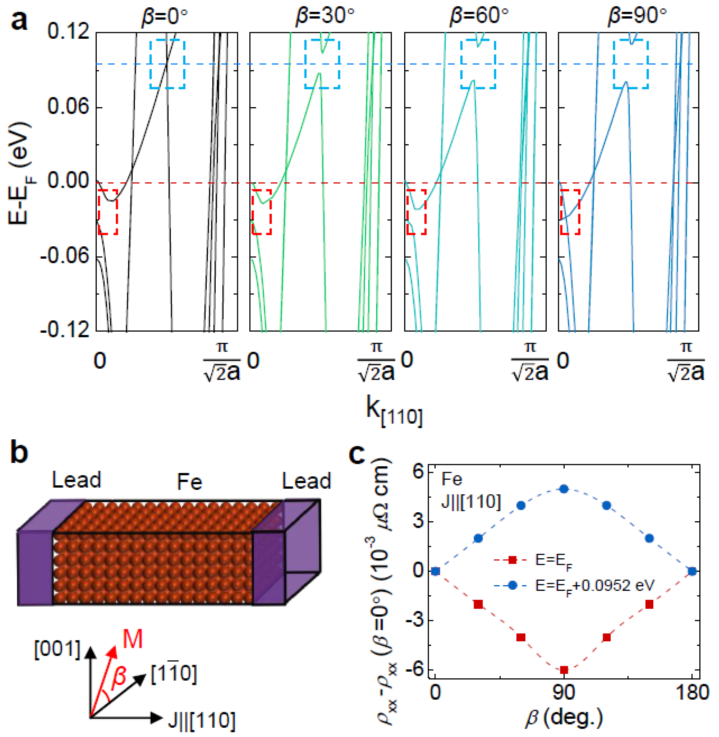


**Fig. S1. The energy-dependent AMR calculated in pure Fe.** (a) Calculated energy bands of body-centered-cubic (bcc) pure Fe along [110] at $\beta = 0°, 30°, 60°$ and $90°$. The $\beta$-dependent bands are marked by red and blue frames. (b) Sketch of the transport geometry with the current along [110]. (c) Calculated resistivity change as a function of $\beta$ at different energies with respect to the real Fermi level. The red and blue symbols indicate the transport calculations performed at the real Fermi level $E_F$ or artificially lifted Fermi energy $E_F$+0.0952 eV.

For simplicity, we calculate the band structure of pure Fe along [110] direction with different magnetization orientations, as plotted in Fig. S1(a). The definition of the angle $\beta$ is given in Fig. S1(b). Near the Fermi energy, we find only two band gaps changed by varying $\beta$, which are related

to two nodal lines and marked by the red and blue frames. In the red frame that is slightly below the Fermi energy, the open gap gradually shrinks for $\beta$ changing from 0° to 90° and eventually becomes a crossing point. Because it is very close to the Fermi level, this special band crossing/anticrossing plays a dominant role in transport. Then we calculate the resistivity $\rho_{xx}$ with **J**||[110] for different $\beta$, as schematically illustrated in Fig. S1(b). The calculated resistivity is plotted by red symbols in Fig. S1(c) as a function of $\beta$ and exhibits its maximum and minimum at $\beta = 0°$ and 90°, respectively. This $\beta$ dependence is consistent with our expectation that the presence of the band crossing (the nodal line) decreases the longitudinal resistivity. The other nodal line in the band structure, marked by the blue frame, is located at a higher energy of ~0.095 eV above the Fermi level. It is a crossing at $\beta = 0°$ but becomes an open gap at $\beta = 90°$. Then, if we artificially shift the Fermi energy to +0.0952eV, the calculated resistivity exhibits a minimum (maximum) at $\beta = 0°$ (90°), as shown by the blue symbols in Fig. S1(c). The above calculations unambiguously demonstrate the correlation between the AMR and the change of band crossing by rotating the magnetization.

The conventional AMR theory already noticed that the band structure should be modified by the magnetization orientation. For instance, the anisotropic *s*-*d* scattering rate was attributed to the $d_{\uparrow}$-$d_{\downarrow}$ mixing [S7], which depends on the quantization axis or magnetization direction of the ferromagnetic metal. Our band structure calculations confirm that this magnetization-orientation-dependence of electronic states arises from the topological nodal line states, which only exist with the demanded symmetry.

**III. Additional analysis for the angular dependent resistivity of $Co_{0.5}Fe_{0.5}$**

The band structure shown in the Fig. 2 of the main text illustrates the strong anisotropy in resistivity along [100] and the weak anisotropy [110] by varying the angle $\alpha$. For **J**||[100], the angle $\alpha$ is also equivalent to $\gamma$. In this section, we illustrate the key changes in band structure by varying the other angles to provide a comprehensive understanding of the angular dependence of resistivity plotted in Fig. 1(c) and (d).

The calculated band structures of Fe and Co for $Co_{0.5}Fe_{0.5}$ along the [100] direction are plotted in Fig. S2, where the Fe band crossing at 0.2 eV above $E_F$ is invariant with $\beta$. In fact it belongs to

a continuous nodal line for $\beta = 0°$ and $90°$, but is an isolated Weyl point for other values of $\beta$. Therefore, the resistivity for J||[100] with an arbitrary $\beta$ is relatively low due to the presence of such a topological state. The weak four-fold symmetry can be attributed to minor band variation below the Fermi level, which exhibits a four-fold symmetry, as highlighted by the red frame in Fig. S2(a). The band structure of Co does not change by rotating $\beta$.

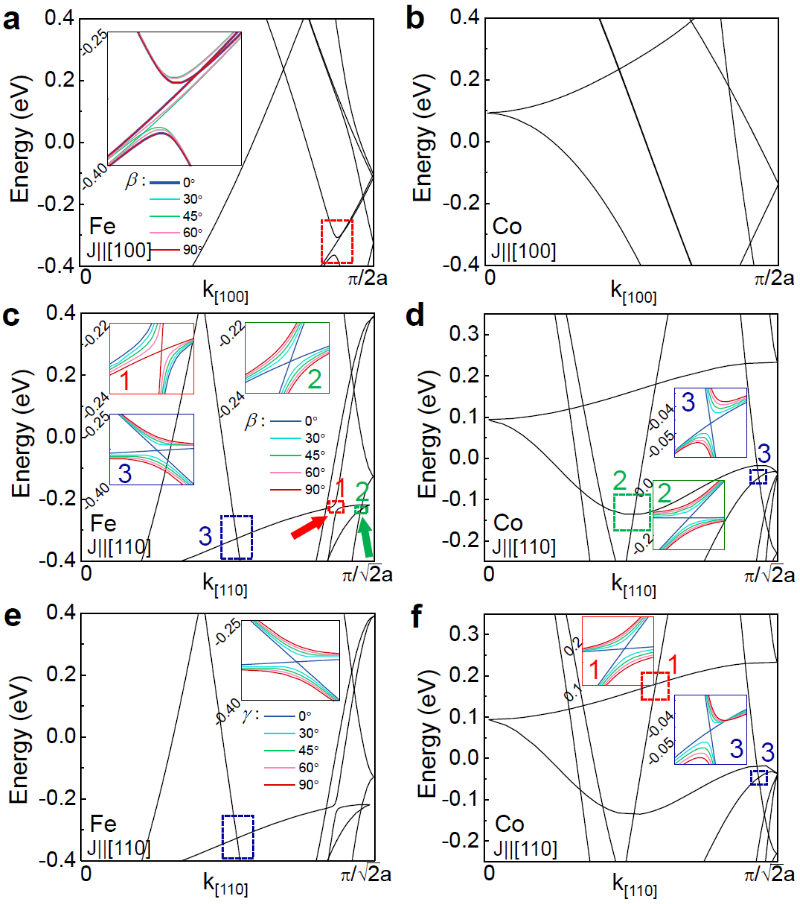

**Fig. S2 Band structure of Fe and Co for $Co_{0.5}Fe_{0.5}$ for different magnetization directions.** The presented bands of Fe and Co are (a-b) along [100] for $\beta$ scan, (c-d) along [110] for $\beta$ scan, and (e-f) along [110] for $\gamma$ scan. The energy bands that change with the varying particular angle are magnified in the insets. The energy bands in the inset of (a) exhibit a four-fold symmetry, i.e. the bands for $\beta = 0°$ and $90°$ are the same. So are those for $\beta = 30°$ and $60°$.

For **J**||[110], the weak AMR with rotating $\alpha$ arises from the band crossing/anticrossing that have opposite angular dependence. The two topological states in the Co band structure never simultaneously exist for any $\alpha$ resulting in the high resistivity. Nevertheless, at $\beta = 0°$, both the two crossings in the Co band structure are present, as shown in Fig. S2(d). For $\beta > 0°$, only one

gap is opened at the crossing point slightly below the Fermi level, as marked by the green frame in Fig. S2(d). As a consequence, the resistivity increases with increasing $\beta$ approaching its maximum at $\beta = 90°$. This is the dominant factor for the observed strong AMR with the angle $\beta$ at **J**||[110]. There are some other $\beta$-dependent bands shown in Fig. S2(c) and (d), which either have relatively small gaps or are located relatively far from the Fermi level and therefore merely have minor effects on AMR.

For **J**||[110] and varying the angle $\gamma$, the other band crossing in Co located slightly above the Fermi level disappears at $\gamma > 0°$ and approaches to the maximum gap at $\gamma = 90°$. The opening gap leads to the strong increase in the resistivity as a function of $\gamma$ from $0°$ to $90°$; see Fig. S2(f). In fact, the two crossing points in Co bands both belong to nodal lines. The low-energy nodal line is essentially the same as that in Fe bands, which is plotted in Fig. 2(c) in the main text. Because Co has a larger number of valence electrons, this nodal line is partially occupied. Therefore, all the angular dependence of the resistivity shown in Fig. 1(c) and (d) in the main text can be well explained by the formation of band crossing/anticrossing.

**IV. Physical origin of the Co concentration dependence**

To further examine the variation of the band crossing with Co concentration, we plot in Fig. S3 the calculated energy bands at different Co concentrations, $x$=0, 0.06, 0.25, 0.5, 0.75 and 1. The cases of $x$=0 and 1 correspond to pure Fe and pure Co, respectively. All the band structures are obtained with the same $k$ ([100] or [110]) direction and perfect crystalline bcc structure but the self-consistent Fe or Co potentials within the coherent potential approximation in $Co_xFe_{1-x}$ alloy are respectively placed on the bcc sites. In Fig. S3(a), the gap in the band along [100] at the energy of 0.45 eV above $E_F$ at $x$=0 first slightly increases and then gradually shifts towards the Fermi level as increasing the Co concentration. This gap will be closed and become a band crossing by rotating magnetization, which can influence the electron scattering and result in AMR. As this gap approaches the Fermi level, it plays the more and more important role in the AMR effect for current along [100], so the calculated AMR ratio is significantly enhanced by increasing $x$. It again indicates the correlation between the AMR and the band crossing modified by the magnetization orientation. It is interesting to note that the calculated AMR exhibits a maximum around $x$=0.5. Although the

crossing point is even closer to the Fermi energy for $x$=0.75, the AMR becomes weaker because of the decrease of Fe concentration in the alloy. The bands along [110] also shift downwards while increasing the Co concentration $x$, as shown in Fig. S3(c) and (d), and both Fe and Co bands have two crossings/anticrossings with opposite magnetization-orientation dependences. Thus, the calculated band structure suggests that the AMR effect with the current along [110] is weak for the whole Co concentration range, in agreement with both the transport calculation and experiment.

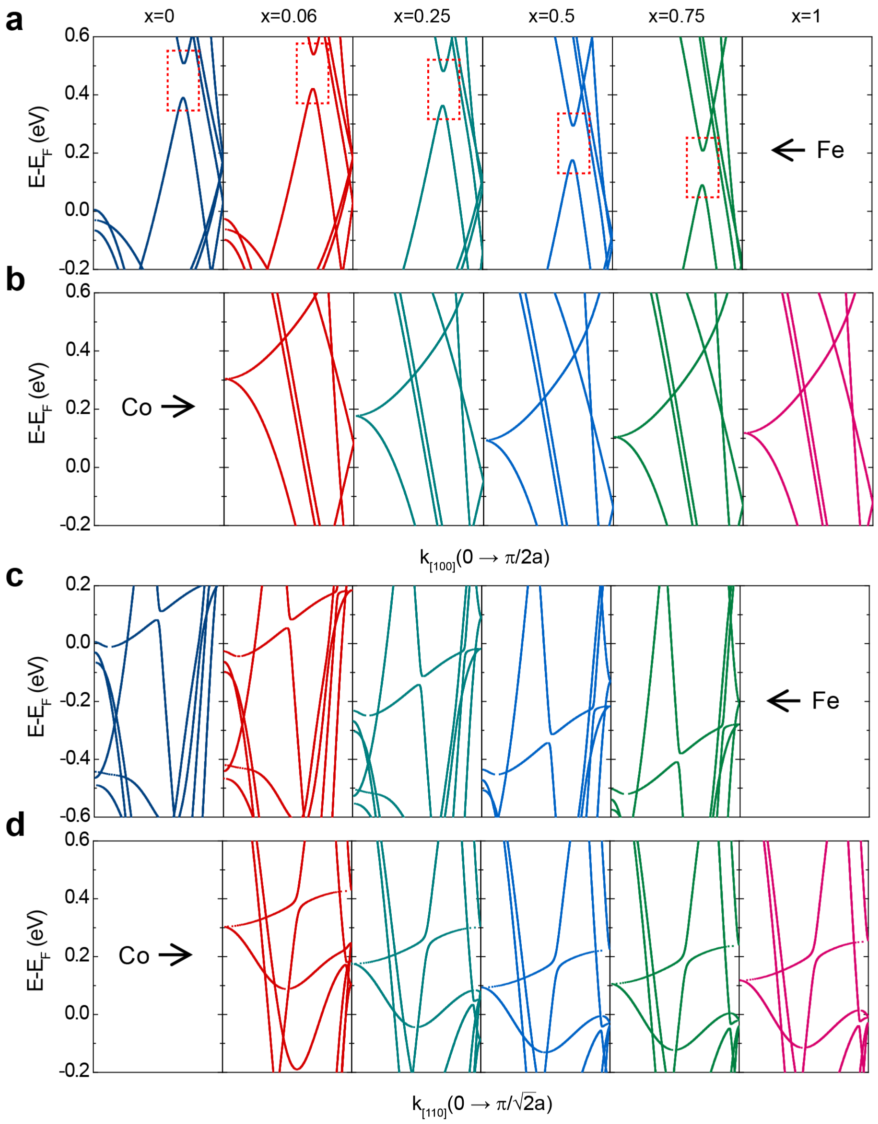


**Fig. S3. Co concentration dependent band structure**. Calculated band structures of Fe (a and c) and Co (b and d) in the $Co_xFe_{1-x}$ alloy with different Co concentration $x$=0, 0.06, 0.25, 0.5, 0.75 and 1 (from left to right) along [100] (a and b) and along [110] (c and d).

Here we take the crossing point in the band structure in Fig. S3(a) as an example, and quantitatively reproduce its energy shift with varying the alloy concentration due to two effects: the density of valence electrons and the exchange splitting. With increasing the Co concentration, the valence electron density monotonically increases and so does the Fermi energy, as shown by the red squares in Fig. S4(a). Then the band crossing points above $E_F$ move downwards. At the same time, the magnetic moments of the $Co_xFe_{1-x}$ alloy also depend on the alloy concentration, which are plotted in the inset of Fig. S4(a). The total magnetic moment has a maximum value at x=0.2 while that of Fe increases monotonically with $x$. The calculated exchange splitting $\Delta E_{ex}$ of Fe bands [S8, S9] exhibits the same dependence, which lifts the minority-spin bands upwards with increasing $x$. Therefore, the total energy shift is determined by $\Delta E_{ex}-E_F$ for the band anticrossing shown in Fig. S3(a) since it belongs to the minority-spin bands of Fe. As shown in Fig. S4(b), the energy of band anticrossing (the black squares) is in perfect agreement with the change in $\Delta E_{ex}-E_F$ (the purple circles). The alloy disorder may vary the energy of the topological states or redistribute them in the reciprocal space, but disorder can not annihilate these states unless the symmetry of the materials is broken [S10].

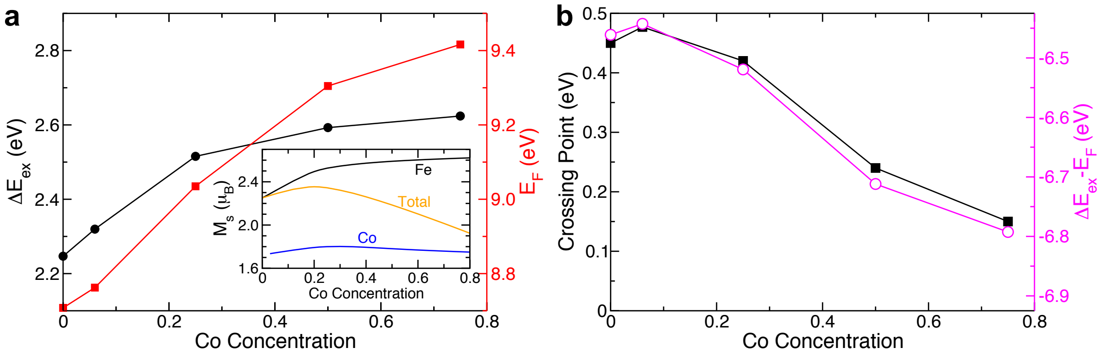


**Fig. S4. Reproducing concentration dependence of (anti)crossing point.** (a) Calculated exchange splitting near the Fermi energy (black circles) and calculated Fermi energy with respect to the bottom of majority valence band (red squares) as a function of Co concentration. Inset: calculated magnetic moments. (b) Energy of (anti)crossing point shown in Fig. S3(a) (black squares). They are quantitatively reproduced by $\Delta E_{ex}-E_F$ (purple circles).

## V. Body-centered-cubic structure of epitaxial $Co_xFe_{1-x}$ film and AMR measurement

The stable structure of Fe is bcc, and that of Co is face-centered-cubic (fcc). Thus, a phase transition is expected from bcc to fcc in $Co_xFe_{1-x}$ alloy with increasing Co concentration and the critical composition $x$ is ~0.70 [S11]. The single-crystal $Co_xFe_{1-x}$/MgO films ($x \leq 0.65$) were prepared by molecular beam epitaxy in an ultrahigh vacuum chamber. The MgO(001) single-crystal substrates were first annealed at 650°C for half an hour. Then a 10-nm-thick MgO seed layer was grown on the substrate at 500 °C. The 10-nm-thick $Co_xFe_{1-x}$ alloy films were deposited via co-evaporation using Fe and Co sources at room temperature. The Fe and Co deposition rates were determined by a quartz thickness monitor, which was calibrated by X-ray reflectometry. During the growth, the film structure can be monitored by *in-situ* reflective high energy electron diffraction (RHEED). Figure S5(a) and (b) display the RHEED patterns of the MgO(001) substrate and 10-nm-thick $Co_{0.65}Fe_{0.35}$ film, where the sharp RHEED patterns confirm the high quality of single crystalline $Co_xFe_{1-x}$ films for $x$ up to 0.65. Due to the commensurate lattice constants of $Co_xFe_{1-x}$ (~2.8 Å) and MgO (4.212 Å), the epitaxial relationship is $Co_xFe_{1-x}$(001)[100] || MgO(001)[110], which is also confirmed by the RHEED patterns. Figure S5 (c) shows the typical X-ray diffraction spectrum of $Co_{0.65}Fe_{0.35}$, $Co_{0.5}Fe_{0.5}$ and $Co_{0.25}Fe_{0.75}$ films, and only $Co_xFe_{1-x}$(002) peak can be observed for all the films with $x \leq 0.65$. The lattice constant of $Co_xFe_{1-x}$ should decrease with increasing $x$, thus the diffraction peak shifts to higher angle for $Co_{0.65}Fe_{0.35}$, which means that the real structure of $Co_xFe_{1-x}$ film is body-centered-tetragonal, not perfect bcc. Before being taken out from the ultrahigh vacuum, the samples were covered with a 6-nm-thick MgO capping layer to prevent oxidation.

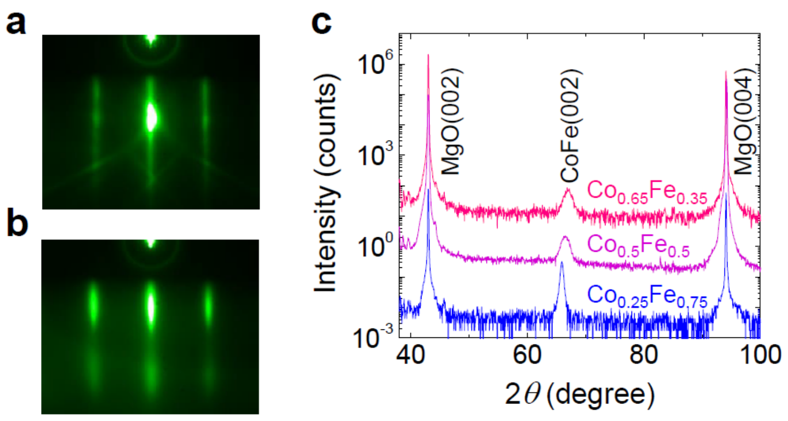


**Fig. S5. Structure characterization of the $Co_xFe_{1-x}$ films.** RHEED patterns of (a) a MgO(001) substrate and (b) a 10-nm-thick $Co_{0.65}Fe_{0.35}$(001) film with the incident electron along the MgO

<100> direction. (c) The X-ray diffractions of a 10-nm-thick $Co_{0.65}Fe_{0.35}$(001), 10-nm-thick $Co_{0.5}Fe_{0.5}$(001) and a 50-nm-thick $Co_{0.25}Fe_{0.75}$(001) film grown on MgO(001) substrate.

For the AMR measurements, standard Hall bars were fabricated with different current orientations by photolithography and lift-off techniques. The Hall bars were 100-μm wide, while the distance between the electrodes was 300 μm. The contacts were made of a 10-nm-thick Cr layer covered by a 30-nm-thick Au film. The out-of-plane AMR was carried out in the Quantum Design Physical Properties Measurement System (PPMS). The sample was rotated out-of-plane under a static magnetic field. The in-plane AMR measurement was conducted in a Dewar system. The sample was fixed in an in-plane rotatable magnetic field, which was produced by a vector magnet. A Keithley 6221 current source provided an ac current, and an SR830 lock-in amplifier simultaneously detected the longitudinal and transverse voltages. All the measurements were conducted at room temperature unless stated otherwise.

## VI. Reciprocal relationship of $\boldsymbol{\Delta\rho_{xx}}$ and $\boldsymbol{\Delta\rho_{xy}}$

The resistivity tensor of a single-crystal material can be generally expressed as a series expansion of the directional cosines of the magnetization [S12, S13], i.e.

$$\rho_{ij} = a_{ij} + a_{kij}m_k + a_{klij}m_k m_l + a_{klmij}m_k m_l m_m + a_{klmnij}m_k m_l m_m m_n. \qquad \text{(S1)}$$

Here, we only include the terms up to the fourth order and the subscripts corresponding to orthogonal coordinate axes implying the Einstein summation. According to the Neumann's principle, the expansion coefficients $a_{ij}$,..., $a_{klmnij}$ must obey the $O_h$ symmetry of bcc $Co_xFe_{1-x}$ alloy. Thus, the number of independent coefficients can be significantly reduced by the symmetry operations. The Onsager relation $\rho_{ij}(\mathbf{M}) = \rho_{ji}(-\mathbf{M})$ is used to further restrict the resistivity tensor. A general resistivity tensor for the electric transport within (001) plane is previously derived as [S12, S13]

$$\boldsymbol{\rho}_{\text{cubic}} = (A - B_2 - D)\begin{pmatrix}1 & 0\\ 0 & 1\end{pmatrix} + (2B_2 + 8D)\begin{pmatrix}m_1^2 & 0\\ 0 & m_2^2\end{pmatrix} + 2B_1\begin{pmatrix}0 & m_1m_2\\ m_1m_2 & 0\end{pmatrix}$$
$$-8D\begin{pmatrix}m_1^4 & 0\\ 0 & m_2^4\end{pmatrix} + 2E\begin{pmatrix}m_2^2m_3^2 & 0\\ 0 & m_3^2m_1^2\end{pmatrix} + 2F\begin{pmatrix}0 & m_1m_2m_3^2\\ m_1m_2m_3^2 & 0\end{pmatrix}, \qquad \text{(S2)}$$

where $m_i$ ($i$=1, 2, 3) are the direction cosines of the magnetization with respect to [100], [010] and [001] crystal directions, respectively. The coefficients $A$, $B_1$, $B_2$, $D$, $E$ and $F$ are combinations of the expansion coefficients in Eq. (S1),

$A = a_{11} + (a_{1111} + a_{1122})/2 + (3a_{111111} + 3a_{111122} + a_{112211})/8,$

$B_1 = (a_{2323} + a_{111212})/2,$

$B_2 = (a_{1111} - a_{1122} + a_{111111} - a_{111122})/2,$

$D = (-a_{111111} - a_{111122} + a_{112211})/8.$

$E = (a_{112233} - 2a_{111122})/2,$

$F = (a_{112323} - a_{111212})/2,$ (S3)

Now we consider the measurement in Fig. 4 of the main text, where the longitudinal and transverse resistivities are obtained with an in-plane magnetization. Following the Ohm's law, we have the electric field $\boldsymbol{E} = \boldsymbol{\rho}(\boldsymbol{M}) \cdot \boldsymbol{J}$, where $\boldsymbol{\rho}(\boldsymbol{M})$ is the resistivity tensor and $\boldsymbol{J}$ is the current. If the principal axes are defined as $x$ ||[100], $y$ ||[010] and $z$ ||[001], the projected two-dimensional resistivity tensor in $x$-$y$ plane can be generally written as

$$\boldsymbol{\rho}^{[100]} = \begin{pmatrix} A + B_2\cos 2\varphi_{\mathrm{M}} - D\cos 4\varphi_{\mathrm{M}} & B_1\sin 2\varphi_{\mathrm{M}} \\ B_1\sin 2\varphi_{\mathrm{M}} & A - B_2\cos 2\varphi_{\mathrm{M}} - D\cos 4\varphi_{\mathrm{M}} \end{pmatrix}, \quad \text{(S4)}$$

where $\varphi_{\mathrm{M}}$ is the angle between the in-plane magnetization $\boldsymbol{M}$ and $\boldsymbol{J}$. Alternatively, if $x$ and $y$ are defined along [110] and $[1\bar{1}0]$, the two-dimensional resistivity tensor reads

$$\boldsymbol{\rho}^{[110]} = \begin{pmatrix} A + B_1\cos 2\varphi_{\mathrm{M}} + D\cos 4\varphi_{\mathrm{M}} & B_2\sin 2\varphi_{\mathrm{M}} \\ B_2\sin 2\varphi_{\mathrm{M}} & A - B_1\cos 2\varphi_{\mathrm{M}} + D\cos 4\varphi_{\mathrm{M}} \end{pmatrix}. \quad \text{(S5)}$$

Equation (S5) essentially can be derived from Eq. (S4) via a unitary transformation. Physically, $A$ is the isotropic resistivity independent of $\boldsymbol{M}$. The leading-order $\boldsymbol{M}$-dependence (two-fold symmetry) of $\rho_{xx}$ and $\rho_{xy}$ results from $B_1$ and $B_2$, respectively. Specifically, at **J**||[100], $B_1$ contributes to $\rho_{xy}$ while $B_2$ is included in $\rho_{xx}$ (AMR). For the other case **J**||[110], $B_1$ contributes to AMR and $B_2$ is responsible for $\rho_{xy}$. In the $Co_xFe_{1-x}$ alloy, the coefficient $D$ is very small and can be neglected. Therefore, $\rho_{xx}$ and $\rho_{xy}$ naturally exhibit the reciprocal relationship, as we observed in experiment.

For an arbitrary direction of the in-plane current, which can be described by an angle $\alpha_{\mathrm{J}}$ between the current and CoFe[110], The longitudinal resistivity $\rho_{xx}(\varphi_{\mathrm{M}}, \alpha_{\mathrm{J}})$ and transverse resistivity $\rho_{xy}(\varphi_{\mathrm{M}}, \alpha_{\mathrm{J}})$ can be further written in the following unifying form,

$$\rho_{xx}(\varphi_{\mathrm{M}}, \alpha_{\mathrm{J}}) = A + B_1\cos 2\alpha_{\mathrm{J}}\cos(2\varphi_{\mathrm{M}} + 2\alpha_{\mathrm{J}}) + B_2\sin 2\alpha_{\mathrm{J}}\sin(2\varphi_{\mathrm{M}} + 2\alpha_{\mathrm{J}}) + D\cos(4\varphi_{\mathrm{M}} + 4\alpha_{\mathrm{J}}), \quad \text{(S6)}$$

$$\rho_{xy}(\varphi_{\mathrm{M}}, \alpha_{\mathrm{J}}) = -B_1\sin 2\alpha_{\mathrm{J}}\cos(2\varphi_{\mathrm{M}} + 2\alpha_{\mathrm{J}}) + B_2\cos 2\alpha_{\mathrm{J}}\sin(2\varphi_{\mathrm{M}} + 2\alpha_{\mathrm{J}}). \quad \text{(S7)}$$

The magnetization angle $\varphi_{\mathrm{M}}$ can be precisely determined by the magnetic anisotropy, which was

quantified through the transverse resistivity measurement [S14]. Therefore, the coefficients $A$, $B_1$, $B_2$ and $D$ can be extracted by fitting the experimental $\rho_{xx(xy)}(\varphi_{\rm M})$ curves with Eqs. (S6) and (S7). Figs. S6(a) and (b) show the experimental curves of $\rho_{xx}(\varphi_{\rm M})$ and $\rho_{xy}(\varphi_{\rm M})$ with the current along [110] ($\alpha_{\rm J} = 0°$) and [100] ($\alpha_{\rm J} = 45°$), which can be well fitted by Eqs. (S6) and (S7). The fitted values of $B_1$, $B_2$, and $D$ as a function of the Co concentration $x$ are plotted in Fig. S6(c). It should be noted that the values of $B_1$ and $B_2$ extracted from the $\rho_{xy}(\varphi_{\rm M})$ curves are systematically larger than those determined from the $\rho_{xx}(\varphi_{\rm M})$ curves, which may be attributed to the effect of the finite electrode size for the $\rho_{xy}$ measurement [S15].

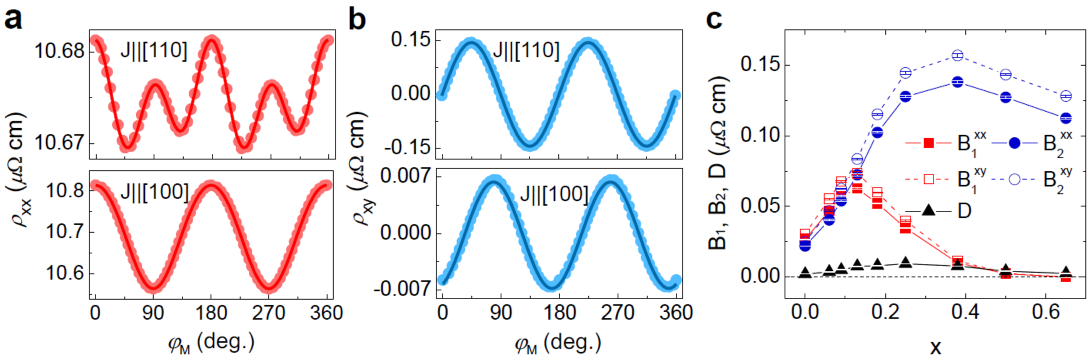


**Fig. S6. Fitting using the phenomenological theory.** (a) and (b) The typical $\rho_{xx}(\varphi_{\rm M})$ (a) and $\rho_{xy}(\varphi_{\rm M})$ (b) curves of a 10 nm $Co_{0.5}Fe_{0.5}$ film with different current directions **J** || [100] and **J** || [100]. The solid lines are the fitting using Eqs. (S6) and (S7). (c) The extracted coefficients $B_1^{xx(xy)}$, $B_2^{xx(xy)}$, and $D$ as a function of $x$.

The fourfold term $D$ is generally one order of magnitude smaller than the twofold term $B_2$. $B_2$ first increases with $x$, then slightly decreases for $x$ above 0.4. $B_1$ first increases along with $x$, but starts to decrease for $x > 0.1$, and becomes vanishingly small for $x > 0.4$. The fact that $B_1 << B_2$ in $Co_{0.5}Fe_{0.5}$ alloy essentially determines that a large (small) AMR ratio is associated with a small (large) transverse resistivity $\rho_{xy}$ at **J** || [100] (**J** || [110]). Therefore, a large current-orientation-dependent AMR generally occurs with $|B_1| << |B_2|$ or $|B_1| >> |B_2|$. For the case of $B_1 = B_2 = B$, Eqs. (S6) and (S7) can be rewritten into $\rho_{xx}(\varphi_{\rm M}, \alpha_{\rm J}) = A + B\cos 2\varphi_{\rm M} + D\cos(4\varphi_{\rm M} + 4\alpha_{\rm J})$ and $\rho_{xy}(\varphi_{\rm M}, \alpha_{\rm J}) = B\sin 2\varphi_{\rm M}$, which reproduces the AMR in polycrystalline films if ignoring the small contribution from $D$. Those expectations are consistent with the experimental measurements for the whole range of the Co concentration $x$: for $x < 0.13$, similar values for $B_1$ and $B_2$ results in a weak

$\alpha_J$-dependent AMR; for $x > 0.2$, a large difference between $B_1$ and $B_2$ leads to a very strong $\alpha_J$-dependence, while the AMR ratio for $\alpha_J = 0°$ nearly vanishes for $x > 0.4$ as the value of $B_1$ is close to zero.

It should be further pointed out that the AMR ratios and $\Delta\rho_{xy}$ curves in Fig. 4 in main text have the in-plane fourfold symmetry, but the principal axis of the AMR ratio switches from <100> to <110>, and the principal axis of $\Delta\rho_{xy}$ switches from <110> to <100> with decreasing Co concentration. This experimental result can be well understood with the above phenomenological model. Since the value of *D* is very small, according to Eqs. (S6) and (S7), we can derive the amplitudes of $\Delta\rho_{xx}$ and $\Delta\rho_{xy}$ with respect to $\alpha_J$ by ignoring *D*:

$$\Delta\rho_{xx}(\alpha_J) \approx \sqrt{\frac{1}{2}(B_1^2 + B_2^2) + \frac{1}{2}(B_1^2 - B_2^2)\cos 4\alpha_J}, \tag{S8}$$

$$\Delta\rho_{xy}(\alpha_J) = \sqrt{\frac{1}{2}(B_1^2 + B_2^2) + \frac{1}{2}(B_1^2 - B_2^2)\cos 4(\alpha_J + 45°)}. \tag{S9}$$

Equations (S8) and (S9) not only explain the 45° offset of the fourfold symmetry axes for $\Delta\rho_{xx}(\alpha_J)$ and $\Delta\rho_{xy}(\alpha_J)$, but also explain the reorientation of the fourfold symmetry axes with decreasing Co concentration. The orientation of the principal axis depends on the sign of $(B_1^2 - B_2^2)$ in Eqs. (S8) and (S9), and our results show that both $B_1$ and $B_2$ depend on the exact composition of the $Co_xFe_{1-x}$ alloy. Fig. S6(c) shows that $B_1 > B_2$ for $x < 0.13$, while $B_1 < B_2$ for $x > 0.13$. Thus, the sign reversal of $(B_1^2 - B_2^2)$ is responsible for the switching of the principal axes from the <100> to <110> direction of the AMR ratio (or from <110> to <100> for $\Delta\rho_{xy}$).

**VII. Additional analysis for the three-dimensional AMR**

In Fig. 3 of the main text, we performed the systematical out-of-plane AMR measurement on a $Co_{0.5}Fe_{0.5}$ device as shown in Fig. 4(a), which was identical with the sample used for the in-plane AMR measurement. The Hall bars have a width of 100 $\mu$m and the voltage electrodes are separated by 300 $\mu$m. The angular-dependent magnetoresistance (ADMR) measurements were carried out in a uniform 9 Tesla field, and the rotation of the sample was controlled by a motorized holder. To characterized the magnetic-field direction with respect to the sample, we define the polar $(\theta_H)$ and azimuthal $(\varphi_H)$ coordinates; see Fig. S7(a). For the standard rotating sample holder, only the one-dimensional polar angle can be adjusted. In our measurement, the sample is rotated for a full circle

of $\theta_{\mathrm{H}}$ with a step of 5° while the resistance is recorded at each step. Then, the sample is taken out and remounted at a different $\varphi_{\mathrm{H}}$ for the next $\theta_{\mathrm{H}}$-dependent ADMR measurement. The above measurement process is repeated for the angle $\varphi_{\mathrm{H}}$ between 0° and 180° with a step of 5°. Figs. S7(b) and (c) show the typical $\theta_{\mathrm{H}}$-dependent resistivity measured at a series of $\varphi_{\mathrm{H}}$ for **J**||[100] and **J**||[110]. Since all the ADMR curves with different $\varphi_{\mathrm{H}}$ contain the same state with $\theta_{\mathrm{H}} = 0°$, so all the measured ADMR curves are offset to ensure the same value of $\rho_{xx}(\theta_{\mathrm{H}} = 0°)$. Figs. S8(a) and (b) show the color plots of the relative AMR as a function of $\theta_{\mathrm{H}}$ and $\varphi_{\mathrm{H}}$ for **J**||[100] and **J**||[110], respectively. The corresponding three-dimensional AMRs of these color plots are displayed in Fig. 3(e) and (f) of the main text. The variation amplitude of $\rho_{xx}(\theta_{\mathrm{H}})$ for **J**||[100] reaches the maximum at $\varphi_{\mathrm{H}} = 0°$ and 180°, and becomes negligible at $\varphi_{\mathrm{H}} = 90°$. This result is expected as a normal AMR feature in the most of the ferromagnetic materials. For **J**||[110], however, the $\rho_{xx}(\theta_{\mathrm{H}})$ curves at different $\varphi_{\mathrm{H}}$ are nearly identical indicating a novel AMR feature $\rho_x \approx \rho_y > \rho_z$ as mentioned in the main text.

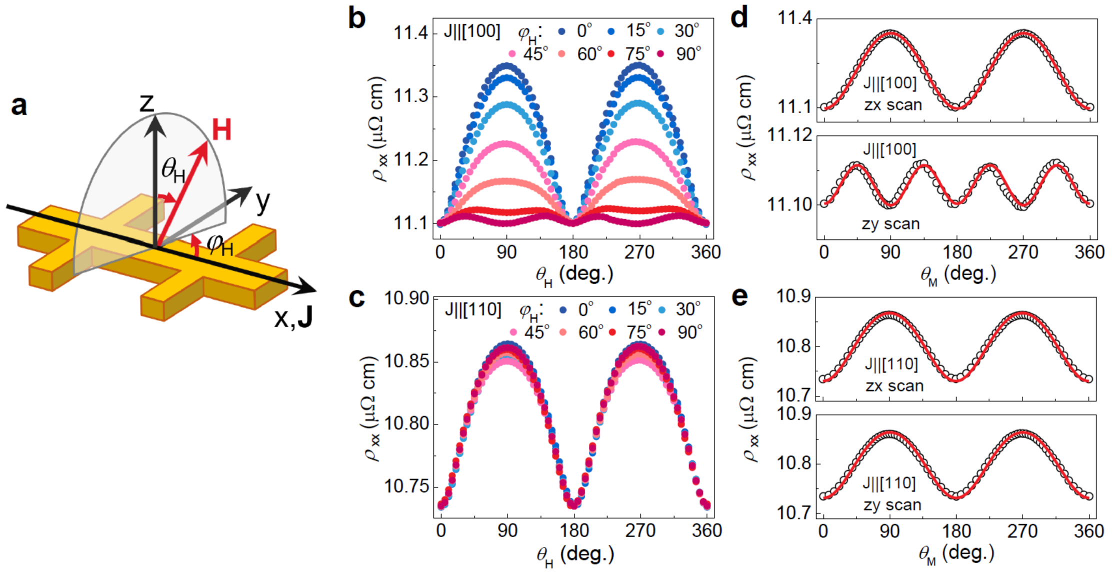


**Fig. S7. Typical three-dimensional AMR results measured for a 10-nm-thick $Co_{0.5}Fe_{0.5}$ sample.** (a) Schematic diagram of the three-dimensional AMR measurement. The current is applied along *x* axis. $\theta_{\mathrm{H}}$ denotes the angle between the magnetic field and *z* axis, and $\varphi_{\mathrm{H}}$ denotes the angle between the current and the projection direction of the magnetic field in *xy* plane. Measured $\theta_{\mathrm{H}}$-dependent resistivity under a 9 Tesla field for (b) **J**||[100] and (c) **J**||[110] with $\varphi_{\mathrm{H}}$ varying from 0° to 90°. The $\theta_{\mathrm{M}}$ dependent resistivity for (d) **J**||[100] and (e) **J**||[110] with the magnetization rotating in the *xz* and *yz* planes. The solid lines in (d) and (e) are the fitting using Eqs. (S12)-(S15).

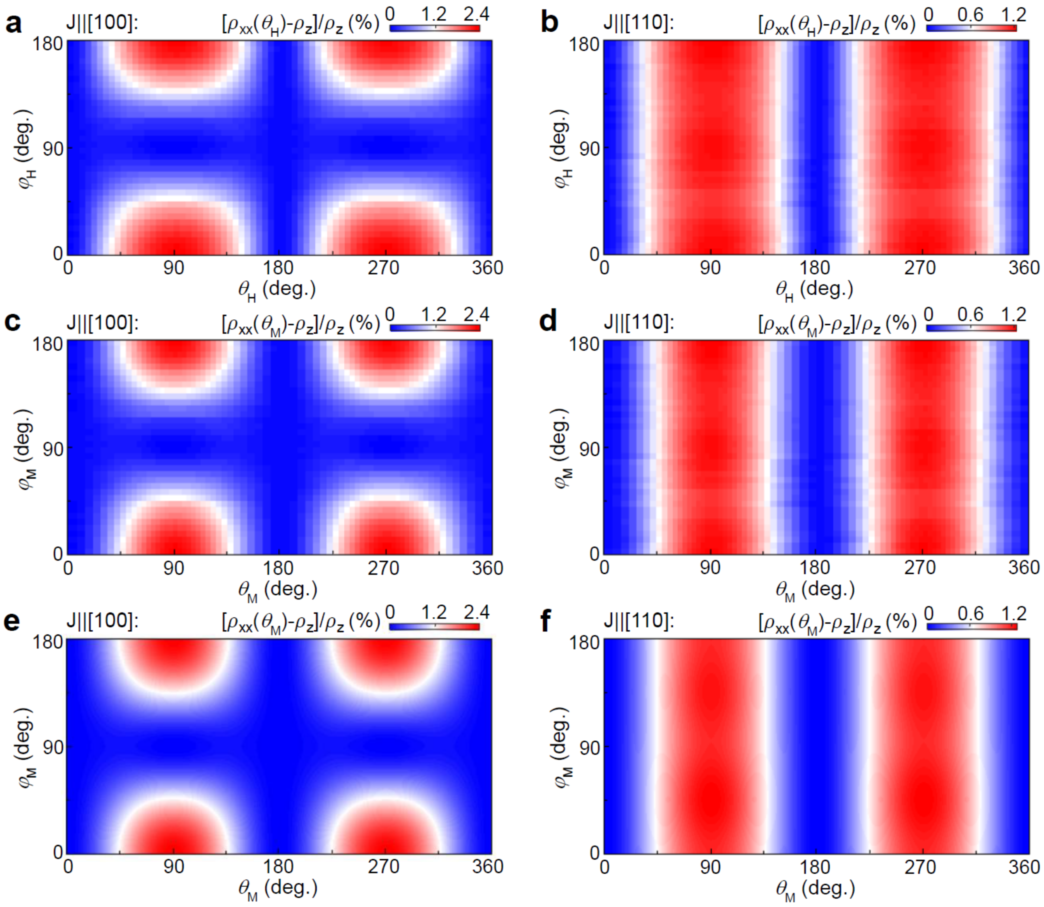


**Fig. S8. Two-dimensional color plot of the three-dimensional AMR of $Co_{0.5}Fe_{0.5}$.** Color plot of measured AMR as a function of $\theta_{\mathrm{H}}$ and $\varphi_{\mathrm{H}}$ for (a) **J**||[100] and (b) **J**||[110]. (c) and (d) Color plots in which the magnetic-field direction is converted to the magnetization orientation. Color plots of calculated AMR for (e) **J**||[100] and (f) **J**||[110] using Eqs. (S10) and (S11) with the coefficients extracted in Figs. S6 and S7.

We further analyzed the out-of-plane AMR using the phenomenological theory. Firstly, it should be noted that, due to the large shape anisotropy, the magnetization cannot be perfectly aligned with the magnetic field. To obtain $\theta_{\mathrm{M}}$ at each $\theta_{\mathrm{H}}$, we extracted the $\theta_{\mathrm{H}}$-dependent anomalous Hall signal $\rho_{\mathrm{AH}}(\theta_{\mathrm{H}})$ from the measured transverse resistivity $\rho_{xy}$ under a 9 Tesla field. In order to rule out the influence of the planar Hall contribution, the AHE signal was determined by $\rho_{\mathrm{AH}}(\theta_{\mathrm{H}})$=$[\rho_{xy}(\theta_{\mathrm{H}}) + \rho_{xy}(\theta_{\mathrm{H}} + 180°)]/2$. It is well known that $\rho_{\mathrm{AH}}(\theta_{\mathrm{M}}) = \rho_{\mathrm{AH}}(0°)\cos\theta_{\mathrm{M}}$, thus the relation between $\theta_{\mathrm{H}}$ and $\theta_{\mathrm{M}}$ can be determined through the curve of $\rho_{\mathrm{AH}}(\theta_{\mathrm{H}})$. Due to the strong field of 9 T applied, we assume that $\varphi_M$ is always equal to $\varphi_H$, then the $\rho_{xx}(\theta_{\mathrm{M}}, \varphi_{\mathrm{M}})$ data

shown in Figs. S8(a) and (b) can be converted to $\rho_{xx}(\theta_\mathrm{M}, \varphi_\mathrm{M})$, which are plotted in Figs. S8(c) and (d).

According to the resistivity tensor in Eq. (S2), a general expression of resistivity for the spatial magnetization direction can be derived. Here, the three-dimensional AMR measurement is done in a simpler case where the current flows along [100] and [110]. The corresponding resistivity can be written as

$$\rho_{xx}^{[100]}(\theta_\mathrm{M}, \varphi_\mathrm{M}) = A - B_2 - D + [B_2 + 4D + E + (B_2 + 4D - E)\cos 2\varphi_\mathrm{M}]\sin^2\theta_\mathrm{M}$$
$$-[3D + E + (4D - E)\cos 2\varphi_\mathrm{M} + D\cos 4\varphi_\mathrm{M}]\sin^4\theta_\mathrm{M}, \quad \text{(S10)}$$
$$\rho_{xx}^{[110]}(\theta_\mathrm{M}, \varphi_\mathrm{M}) = A - B_2 - D + [B_2 + 4D + E + (B_1 + F)\cos 2\varphi_\mathrm{M}]\sin^2\theta_\mathrm{M}$$
$$-(3D + E + F\cos 2\varphi_\mathrm{M} - \mathrm{D}\cos 4\varphi_\mathrm{M})\sin^4\theta_\mathrm{M}. \quad \text{(S11)}$$

Note the coefficients $A$, $B_1$, $B_2$ and $D$ has been obtained in the in-plane AMR measurement, $B_1$=2.3 nΩ cm, $B_2$=127.3 nΩ cm and $D$=4.2 nΩ cm at $x$=0.5, as shown in Fig. S6(c). The remaining coefficients $E$ and $F$ can be extracted from additional out-of-plane rotations. With the magnetization rotating in the *xz* or *yz* plane, the resistivity $\rho_{xx}(\theta_\mathrm{M}, \varphi_\mathrm{M})$ is written as

$$\rho_{xx}^{[100]}(\theta_\mathrm{M}, 0°) = A - B_2 - D + (2B_2 + 8D)\sin^2\theta_\mathrm{M} - 8D\sin^4\theta_\mathrm{M}, \quad \text{(S12)}$$
$$\rho_{xx}^{[100]}(\theta_\mathrm{M}, 90°) = A - B_2 - D + 2E\sin^2\theta_\mathrm{M} - 2E\sin^4\theta_\mathrm{M}, \quad \text{(S13)}$$
$$\rho_{xx}^{[110]}(\theta_\mathrm{M}, 0°) = A - B_2 - D + (B_2 + 4D + E + B_1 + F)\sin^2\theta_\mathrm{M} - (2D + E + F)\sin^4\theta_\mathrm{M}, \quad \text{(S14)}$$
$$\rho_{xx}^{[110]}(\theta_\mathrm{M}, 90°) = A - B_2 - D + (B_2 + 4D + E - B_1 - F)\sin^2\theta_\mathrm{M} - (2D + E - F)\sin^4\theta_\mathrm{M}. \quad \text{(S15)}$$

For **J**||[100], the $\theta_\mathrm{M}$-dependence of $\rho_{xx}^{[100]}$ in the *zx* scan can be well reproduced by Eq. (S12) with the $B_2$ and $D$ values obtained in the *xy* scan, as shown in Fig. S7(d). The parameter $E$ can be extracted from the $\rho_{xx}^{[100]}(\theta_\mathrm{M}, 90°)$ curve, since Eq. (S13) can be rewritten as $\rho_{xx}^{[100]} = A - B_2 - D + E/4 - E/4 \cdot \cos 4\theta_\mathrm{M}$. By fitting the curve with a four-fold symmetry in Fig. S7(d), we obtain $E$=19.5 nΩ cm. Finally, the curve $\rho_{xx}^{[110]}(\theta_\mathrm{M}, 0°)$ in the *zx* scan for **J**||[110] [see Fig. S7(e)] is used to determine $F$ by fitting the curve with Eq.(S14), and the resulted value is $F$=2.8 nΩ·cm. Using the determined parameters $A$, $B_1$, $B_2$, $D$, $E$ and $F$, we can calculate the $\rho_{xx}^{[110]}(\theta_\mathrm{M},90°)$ curve, which well agrees with the experimental curve of $\rho_{xx}^{[110]}(\theta_\mathrm{M},90°)$, as shown in Fig. S7(e).

To further verify the validity of these extracted coefficients, we calculate the three-dimensional AMR $\rho_{xx}(\theta_\mathrm{M}, \varphi_\mathrm{M})$ by using Eqs. (S10) and (S11) for **J**||[100] and **J**||[110], respectively. The color plots of the calculated AMR in Figs. S8(e) and (f) perfectly reproduce the

angular dependence of experimental AMR in Figs. S8(c) and (d). It should be noted the coefficient $B_2$ is still much larger than other coefficients. Thus, the phenomenological model can well explain that the out-of-plane AMR strongly depends on $\varphi_{\mathrm{M}}$ for **J**||[100] and is nearly independent of $\varphi_{\mathrm{M}}$ for **J**||[110]. Besides, in the calculated results, the maximum amplitude of $\rho_{xx}(\theta_{\mathrm{M}})$ for **J**||[100] is almost twice that for **J**||[110], which is also in consistent with the experimental results.

It should be emphasized that the above phenomenological analysis is based on the perfect cubic symmetry. In section V, the XRD result reveals a slight tetragonal distortion along [001] direction in our $Co_xFe_{1-x}$ samples. This distortion is found to introduce an additional contribution into the resistivity tensor [S16]. The resistivity tensors for tetragonal symmetry can be expressed as $\boldsymbol{\rho}_{\text{tetragonal}} = \boldsymbol{\rho}_{\text{cubic}} + \Delta\boldsymbol{\rho}$, where the additional resistivity reads [S16]

$$\Delta\boldsymbol{\rho} = \begin{pmatrix} -bm_3^2 & 0 \\ 0 & -bm_3^2 \end{pmatrix} + \begin{pmatrix} 2em_2^2m_3^2 - dm_3^4 & 2fm_1m_2m_3^2 \\ 2fm_1m_2m_3^2 & 2em_3^2m_1^2 - dm_3^4 \end{pmatrix}. \tag{S16}$$

Here we have four additional coefficients, which are given by

$b = a_{1122} - a_{3311} + 6a_{112211} - 6a_{113311}$,

$d = a_{111122} - 6a_{112211} + 6a_{113311} - a_{333311}$,

$e = 3a_{113322} - 3a_{112233} + 3a_{112211} - 6a_{113311}$,

$f = 6a_{123312} - 6a_{112323}$.

Since the $m_3$ term in Eq. (S16) should be zero for the in-plane AMR measurement, $\Delta\boldsymbol{\rho}$ does not contribute to the in-plane AMR expressions in Eqs. (S6) and (S7). Combining Eqs. (S2) and (S16), we can rewrite Eqs. (S10) and (S11) as

$$\left(\rho_{xx}^{[100]}\right)'(\theta_{\mathrm{M}}, \varphi_{\mathrm{M}}) = A - B_2' - D - d + [B_2' + 4D + 2d + E' + (B_2 + 4D - E')\cos 2\varphi_{\mathrm{M}}]\sin^2\theta_{\mathrm{M}} \\ -[3D + d + E' + (4D - E')\cos 2\varphi_{\mathrm{M}} + D\cos 4\varphi_{\mathrm{M}}]\sin^4\theta_{\mathrm{M}}, \tag{S17}$$

$$\left(\rho_{xx}^{[110]}\right)'(\theta_{\mathrm{M}}, \varphi_{\mathrm{M}}) = A - B_2' - D - d + [B_2' + 4D + 2d + E' + (B_1 + F')\cos 2\varphi_{\mathrm{M}}]\sin^2\theta_{\mathrm{M}} \\ -(3D + d + E' + F'\cos 2\varphi_{\mathrm{M}} - D\cos 4\varphi_{\mathrm{M}})\sin^4\theta_{\mathrm{M}}, \tag{S18}$$

with the abbreviations $B_2' = B_2 + b$, $E' = E + e/2$, and $F' = F + f/2$. The expressions $\left(\rho_{xx}^{[100]}\right)'$ and $\left(\rho_{xx}^{[110]}\right)'$ show very similar forms of $\rho_{xx}^{[100]}$ and $\rho_{xx}^{[110]}$ in Eqs. (S10) and (S11), so it is difficult to precisely extract the numerical values of the additional parameters $b$, $d$, e and $f$ induced by the tetragonal lattice distortion. On the other hand, since Eqs. (S10) and (S11) base on the cubic symmetry can well describe the measured three-dimensional AMR shown in Fig. S8(c)

and (d), we expect that the tetragonal distortion of the epitaxial CoFe film has very little influence on the quantitative values fitted based on the phenomenological theory with the cubic structure.

## VIII. Quantitative comparison of the intrinsic AMR

The proposed intrinsic mechanism for AMR is a pure band effect, which only depends on the change of band structure with rotating the magnetization direction. Therefore, the sample thickness or environmental temperature, which determines the momentum relaxation time in electronic transport, becomes less important. We perform a quantitative comparison between experimental measurement and theoretical calculation to verify the prediction.

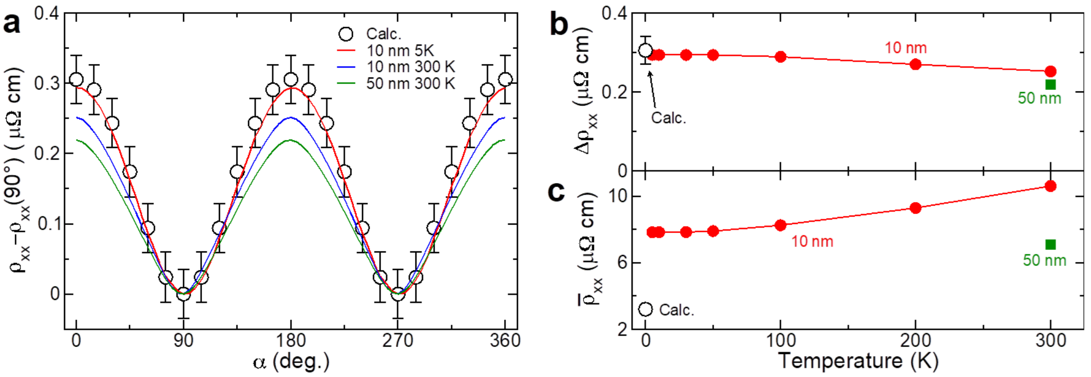


**Fig. S9 Experimental and calculated resistivity variation of $Co_{0.5}Fe_{0.5}$.** (a) Variation in resistivity as a function of magnetization direction. The angle $\alpha$ is defined in Fig. 1(b) of the main text. The circles are the calculated values for bulk $Co_{0.5}Fe_{0.5}$, while the lines are experimental values for a 10-nm-thick sample at low temperature (red) and room temperature (blue) and for a 50-nm-thick sample at room temperature (green). Calculated and experimental resistivity variation (b) and average resistivity (c) as a function of temperature. The empty circles represent the calculated values.

Figure S9(a) shows the resistivity variation $\rho_{xx}(\alpha) - \min[\rho_{xx}(\alpha)]$ as a function of the angle $\alpha$, which is defined in Fig. 1(b) of the main text. The experimental values that are measured for different samples and temperatures are in quantitative agreement with the calculated resistivity variation for the bulk alloy. On the other hand, the absolute values of the resistivity show large dispersion: the averaged resistivity over all angles of the 10-nm-thick sample is $\bar{\rho}_{xx} = 7.8\ \mu\Omega$ cm at 5 K, and it increases to 10.6 $\mu\Omega$ cm at 300 K while the value of the 50-nm-thick sample is about 7.1 $\mu\Omega$ cm at 300 K. The calculation is done with perfect lattice and collinear magnetization to

simulate the zero-temperature condition and the resulting resistivity is approximately 3.2 $\mu\Omega$ cm; see Fig. S9(c). However, all the resistivity variation $\Delta\rho_{xx}$ is quantitatively consistent with one another, as explicitly illustrated in Fig. S9(b).

Such a surprisingly good agreement indicates that the intrinsic mechanism for AMR is in fact the dominant contribution in the $Co_{0.5}Fe_{0.5}$ alloy. Therefore, the resistivity variation, or the AMR amplitude, arises only from the band structure, e.g. the Fermi velocity, the energy difference between the Fermi energy and the topological states [S17, S18]. The minor effect of temperature can be understood as the resulting fluctuation of the Fermi energy [S18] and/or the excitation of magnons. The latter causes a destructive influence on the formation of topological states due to the locally broken symmetry.

**References:**

[S1] I. Turek, V. Drchal, J. Kudrnovský, M. Sob, P. Weinberger, *Electronic structure of disordered alloys, surfaces and interfaces.* (Kluwer, Boston-London-Dordrecht, 1997).

[S2] A. A. Starikov, Y. Liu, Z. Yuan, P. J. Kelly, *Calculating the transport properties of magnetic materials from first principles including thermal and alloy disorder, noncollinearity, and spin-orbit coupling.* Phys. Rev. B **97**, 214415 (2018).

[S3] P. Khomyakov, G. Brocks, V. Karpan, M. Zwierzycki, and P. J. Kelly, *Conductance calculations for quantum wires and interfaces: Mode matching and Green's functions.* Phys. Rev. B **72**, 035450 (2005).

[S4] H. Ebert, S. Mankovsky, D. Ködderitzsch, and P. J. Kelly, *Ab Initio calculation of the Gilbert damping parameter via the linear response formalism.* Phys. Rev. Lett. **107**, 066603 (2011).

[S5] I. Turek, J. Kudrnovský, and V. Drchal, *Ab initio theory of galvanomagnetic phenomena in ferromagnetic metals and disordered alloys.* Phys. Rev. B **86**, 014405 (2012).

[S6] A. A. Starikov, P. J. Kelly, A. Brataas, Y. Tserkovnyak, and G. E. W. Bauer, *Unified first-principles study of Gilbert damping, spin-flip diffusion, and resistivity in transition metal alloys.* Phys. Rev. Lett. **105**, 236601 (2010).

[S7] I. Campbell, A. Fert, O. Jaoul, *The spontaneous resistivity anisotropy in Ni-based alloys.* J. Phys. C: Solid State Phys. **3**, S95 (1970).

[S8] O. Gunnarsson, *Band model for magnetism of transition metals in the spin-density-functional formalism.* J. Phys. F: Metal Phys. **6**, 587 (1976).

[S9] Z. Yuan and P. J. Kelly, *Spin-orbit-coupling induced torque in ballistic domain walls: Equivalence of charge-pumping and nonequilibrium magnetization formalisms.* Phys. Rev. B **93,** 224415 (2016).

[S10] Y. Su, X. S. Wang and X. R. Wang, *A generic phase between disordered Weyl semimetal and diffusive metal.* Sci. Rep. **7**, 14382 (2017).

[S11] G. Prinz, *Stabilization of bcc Co via epitaxial growth on GaAs.* Phys. Rev. Lett. **54**, 1051 (1985).

[S12] T. McGuire, R. Potter, *Anisotropic magnetoresistance in ferromagnetic 3d alloys.* IEEE Trans. Magn. **11**, 1018–1038 (1975).

[S13] R. R. Birss, *Symmetry and magnetism.* (North-Holland Amsterdam, 1964).

[S14] W. N. Cao, J. Li, G. Chen, J. Zhu, C. R. Hu, Y. Z. Wu, *Temperature-dependent magnetic anisotropies in epitaxial Fe/CoO/MgO(001) system studied by the planar Hall effect.* Appl. Phys. Lett. **98**, 262506 (2011).

[S15] F. L. Zeng, C. Zhou, M. W. Jia, D. Shi, Y. Huo, W. Zhang, Y. Z. Wu, *Strong current-direction dependence of anisotropic magnetoresistance in single crystalline Fe/GaAs(110) films*. J. Magn. Magn. Mater. **499**, 166204 (2020).

[S16] W. Limmer, J. Daeubler, L. Dreher, M. Glunk, W. Schoch, S. Schwaiger, R. Sauer, *Advanced resistivity model for arbitrary magnetization orientation applied to a series of compressive-to tensile-strained (Ga, Mn)As layers*. Phys. Rev. B **77**, 205210 (2008).

[S17] Q. -D. Jiang, H. Jiang, H. Liu, Q. -F. Sun, X. -C. Xie, *Topological Imbert-Fedorov shift in Weyl semimetals*. Phys. Rev. Lett. **115**, 156602 (2015).

[S18] Q. -D. Jiang, H. Jiang, H. Liu, Q. -F. Sun, X. -C. Xie, *Chiral wave-packet scattering in Weyl semimetals*. Phys. Rev. B **93**, 195165 (2016).
